# Supplementary material for: Boosting Reasoning in Large Multimodal Models via Activation Replay
Source: arXiv:2511.19972 source file (2026-08-26)
Supplement: Supplementary file 1 [file fig_seg.tex]

\begin{figure*}[!ht]
    \centering
    \includegraphics[width=\linewidth]{example-image-a}
    \caption{Case Study of Reasoning Segmentation.}
    \label{fig:seg_case}
\end{figure*}
